# Supplementary material for: NarrativeXL: A Large-scale Dataset For Long-Term Memory Models
Source: arXiv:2305.13877 source file (2023-12-08)
Supplement: Supplementary file 1 [file appendix_stats.tex]

\begin{table*}[]
\begin{tabular}{llll}
\textbf{Narrative XL question type} & \textbf{Avg. Words} & \textbf{Memory load} & \textbf{Task Items}       \\ \hline
Read along (train)                          &  &                                          & 726,803 (multiple choice) \\
Read along (test)                          &    &                                      & 726,803 (multiple choice) \\     
\end{tabular}
\caption{NarrativeXL dataset statistics per split. Here memory load denotes how many words ``ago'' the relevant information was presented, hence it is lower than total context length.} \label{tab:narrativexl_stats}
\end{table*}
